# Supplementary material for: Hierarchical Open-Vocabulary 3D Scene Graphs for Language-Grounded Robot Navigation
Source: arXiv:2403.17846 source file (2024-06-03)
Supplement: Supplementary file 1 [file appendix.tex]

\begin{table*}[b]
\centering
\scriptsize
\caption{Object-Level Instance Segmentation and Semantics Evaluation on HM3DSem}
\setlength\tabcolsep{3pt}
\begin{threeparttable}
\begin{tabular}{cc|ccc|cccccccl}
 \toprule

Method & Scene & \multicolumn{3}{c|}{Instance Segmentation} & \multicolumn{7}{c}{Semantics} \\
 \midrule

& Scene & $\text{AP}$ & $\text{P}_{\text{50\%}}^{\text{IoU}}$ & $\text{R}_{\text{50\%}}^{\text{IoU}}$ & $top_{5}$ & $top_{10}$ & $top_{25}$ & $top_{100}$ & $top_{250}$ & $top_{500}$ & AUC$_{k}^{top}$ \\
\midrule
 \multirow{8}{*}{\rotatebox[origin=c]{90}{VLMaps \cite{huang23vlmaps}}} & \textit{00824} & - & - & - & 0.0 & 0.0 & 0.0 & 15.21 & 22.16 & 34.79 & 54.39 \\
  & \textit{00829}  & - & - & - & 0.0 & 0.0 & 0.0 & 19.18 & 34.29 & 48.98 & 61.36 \\
& \textit{00843}  & - & - & - & 0.0 & 0.0 & 0.0 & 15.52 & 27.16 & 45.07 & 57.43 \\
& \textit{00861}  & - & - & - & 0.0 & 0.0 & 1.29 & 18.74 & 29.98 & 44.03 & 60.05 \\
& \textit{00862}  & - & - & - & 0.0 & 0.0 & 0.0 & 17.1 & 25.3 & 37.6 & 56.12 \\
& \textit{00873} & - & - & - & 0.22 & 0.67 & 1.78 & 15.56 & 22.89 & 34.89 & 52.89 \\
& \textit{00877} & - & - & - & 0.2 & 0.4 & 0.6 & 14.0 & 26.8 & 37.4 & 54.03 \\
& \textit{00890} & - & - & - & 0.0 & 0.31 & 0.62 & 7.23 & 19.54 & 37.38 & 53.35 \\
\midrule
\multicolumn{2}{r|}{Overall} & - & - & - & 0.05 & 0.17 & 0.54 & 15.32 & 26.01 & 40.02 & 56.20  \\
 \midrule
\multirow{8}{*}{\rotatebox[origin=c]{90}{ConceptGraphs~\cite{conceptgraphs} % eval using faiss IoU
  }} & \textit{00824} & 23.95 & 41.65 & 48.19 & 21.65 & 29.38 & 35.57 & 57.47 & 72.16 & 82.22 & 84.41 \\ 
 & \textit{00829} & 21.78 & 43.18 & 54.28 & 16.73 & 22.86 & 35.10 & 58.37 & 75.51 & 83.67 & 86.00 \\ 
 & \textit{00843} & 15.20 & 38.58 & 43.88 & 15.52 & 20.30 & 27.76 & 51.34 & 68.96 & 79.10 & 82.05 \\ 
 & \textit{00861} & 15.11 & 36.40 & 33.37 & 10.47 & 14.18 & 21.84 & 39.21 & 60.41 & 74.58 & 79.55 \\ 
 & \textit{00862} & 26.24 & 42.69 & 57.50 & 22.30 & 27.90 & 38.40 & 64.30 & 79.90 & 87.40 & 88.43 \\ 
 & \textit{00873} & 26.71 & 49.81 & 57.11 & 21.33 & 28.00 & 37.55 & 60.44 & 73.11 & 83.11 & 84.35 \\ 
 & \textit{00877} & 26.36 & 51.33 & 46.20 & 21.56 & 27.55 & 36.66 & 55.78 & 68.44 & 81.33 & 83.80 \\ 
 & \textit{00890} & 22.74 & 49.47 & 42.77 & 15.30 & 21.89 & 31.11 & 54.44 & 68.33 & 80.96 & 83.97 \\ 
 \midrule
 \multicolumn{2}{r|}{Overall} & - & - & - & - & - & - & - & - & - & \underline{84.07} \\
 \midrule
\midrule
\multirow{8}{*}{HOV-SG}  & \textit{00824} & 17.58 & 40.46 & 31.70 & 21.38 & 30.59 & 40.13 & 64.14 & 75.66 & 82.24 & 86.52 &\\ % peach field rlsim1
& \textit{00829} & 16.05 & 44.66 & 37.56 & 19.90 & 25.72 & 40.29 & 59.71 & 73.30 & 82.04 & 86.12 \\ % peach field rlsim1
& \textit{00843} & 11.09 & 34.98 & 29.55 & 11.31 & 16.61 & 28.62 & 46.64 & 61.48 & 72.79 & 79.23 \\ % fearless donkey rlsim1
& \textit{00861} & 11.76 & 38.49 & 26.81 & 11.93 & 19.49 & 28.74 & 47.39 & 62.35 & 76.47 & 81.94 \\ % fearless donkey rlsim1
& \textit{00862} & 20.14 & 44.06 & 41.60 & 19.49 & 27.01 & 37.18 & 57.94 & 71.50 & 81.36 & 86.17 \\ % galliant-hill rlsim1
& \textit{00873} & 21.54 & 53.65 & 37.56 & 21.90 & 30.79 & 41.90 & 64.44 & 78.73 & 89.20 & 88.35 \\ % 
& \textit{00877} & 18.91 & 51.10 & 32.40 & 23.02 & 31.54 & 39.11 & 59.62 & 70.34 & 81.80 & 85.33 \\ % genial dream rlsim1
& \textit{00890} & 17.31 & 49.75 & 30.15 & 18.53 & 24.11 & 35.28 & 51.78 & 66.24 & 80.96 & 85.36 \\ % genial dream rlsim1
\midrule
\multicolumn{2}{r|}{Overall (ours)} & - & - & - & - & - & - & - & - & - & \textbf{84.88} \\
\midrule
\bottomrule
\end{tabular}

\begin{table*}[b]
\centering
\scriptsize
\caption{Room and Floor Segmentation Performance on HM3DSem}
\setlength\tabcolsep{3.7pt}
\begin{threeparttable}
\begin{tabular}{cc|ccc|cccccc}
 \toprule

\multirow{2}{*}{Method} & \multirow{2}{*}{Scene}  & \multicolumn{3}{c|}{Floor Segmentation} & \multicolumn{6}{c}{Room Segmentation} \\
 % \cmidrule{3-11}
&  & $\text{Acc}_{F}$ & $\text{F}_{\text{P}}$ & $\text{F}_\text{GT}$ &  
 $\text{P}$ &  $\text{R}$ &  $\text{AP}$ & $\text{Acc}_{\text{50\%}}^{\text{IoU}}$ & $\text{P}_{\text{50\%}}^{\text{IoU}}$ & $\text{R}_{\text{50\%}}^{\text{IoU}}$ \\
 \midrule
\multirow{8}{*}{\rotatebox[origin=c]{90}{HOV-SG (ours)}} & \textit{00824} & 1.0 & 1 & 1 & 81.20 & 80.00 & 70.00 & 70.00 & 100.0 & 70.00 \\ % sunny-pond
& \textit{00829} & 1.0 & 1 & 1 & 88.81 & 88.02 & 71.43 & 71.43 & 100.0 & 71.43 \\ % sunny-pond
& \textit{00843} & 1.0 & 2 & 2 & 88.54 &87.10 & 61.54 & 61.54 & 100.0 & 61.54 \\ % sunny-pond
& \textit{00861} & 1.0 & 2 & 2 & 76.41 & 89.95 & 45.83 & 40.00 & 90.91 & 45.83 \\ % sunny-pond
& \textit{00862} & 1.0 & 3 & 3 & 72.65 & 76.10 & 42.88 & 33.33 & 81.25 & 41.67 \\ % desert-yoghurt
& \textit{00873} & 1.0 & 2 & 2 & 95.63 & 67.71 & 53.54 & 53.85 & 77.78 & 63.64 \\ % lilac-bird
& \textit{00877} & 1.0 & 2 & 2 & 74.82 & 92.30 & 46.15 & 35.71 & 83.33 & 46.15 \\ % lilac-bird
& \textit{00890} & 1.0 & 2 & 2 & 94.75 & 87.55 & 81.81 & 81.81 & 100.0 & 81.81 \\ % ethereal-meadow
\cmidrule{2-11}
& Overall & 1.0 & - & - & - & - & - & - & - & - \\
\midrule
\bottomrule
\end{tabular}

\footnotesize
Evaluation of the floor and room segmentation: Room Segmentation is compared against VLMaps and Hydra while we do not compare the floor segmentation as it use a na\"ive heuristic. We provide the number of correctly predicted floors using a threshold of 0.5m? (\red{check this again @Martin}). Room segmentation precision (P) and recall (R) are calculated based on the metric provided by \citet{hughes2022hydra}.
\end{threeparttable}
\label{tab:seg-ablation}
\end{table*}

\begin{table}[b]
\centering
\scriptsize
\caption{Object Retrieval from Language Queries (HM3DSem)}
\setlength\tabcolsep{2pt}
\begin{threeparttable}
\begin{tabular}{lcccccccc}
 \toprule
Query Type & Scene & \# Floors & \# Rooms & \# Trials & Mean-SR [\%] & Median-SR[\%] & Max-SR$_{25}$[\%] & Max-SR$_{10}$[\%] \\
\midrule
\multirow{9}{*}{(\texttt{o}, \texttt{r}, \texttt{f})} & \textit{00824} & 1 & 10 & 33 & 48.48 & 54.54 & 48.48 & 57.57 \\
 & \textit{00829} & 1 & 7 & 20 & 35.00 & 35.00 & 35.00 & 45.00\\
 & \textit{00843} & 2 & 13 & 26 & 34.62 & 34.62 & 30.77 & 34.62 \\
 & \textit{00861} & 2 & 24 & 55 & 10.91 & 12.73 & 16.36 & 25.45 \\
 & \textit{00862} & 3 & 36 & 90 & 13.33 & 14.44 & 20.00 & 21.11 \\
 & \textit{00873} & 2 & 11 & 28 & 07.14 & 07.14 & 14.29 & 14.29 \\
 & \textit{00877} & 2 & 13 & 32 & 25.00 & 25.00 & 25.00 & 25.00 \\
 & \textit{00890} & 2 & 11 & 41 & 19.51 & 19.51 & 19.51 & 21.95 \\
 \cmidrule{2-9}
  & \textit{Overall} &  & & & 20.92 & 22.15 & 24.00 & 28.00 \\
 \midrule
\multirow{8}{*}{(\texttt{o}, \texttt{r})} & \textit{00824} & 1 & 10 & 33 &  &  & 48.48 & 57.58 \\
 & \textit{00829} & 1 & 7 & 20 & - & - & 35.00 & 45.00 \\
 & \textit{00843} & 2 & 13 & 23 & - & - & 34.78 & 39.13\\
 & \textit{00861} & 2 & 24 & 46 & - & - & 19.57 & 30.43\\
 & \textit{00862} & 3 & 36 & 67 &  &  & 20.63 & 20.63\\
 & \textit{00873} & 2 & 11 & 25 & - & - & 20.00 & 20.0\\
 & \textit{00877} & 2 & 13 & 24 & - & - & 33.33 & 33.33\\
 & \textit{00890} & 2 & 11 & 41 & - & - & 19.51 & 21.95\\
  \cmidrule{2-9}
  & \textit{Overall} &  & & & - & - & 27.04 & 31.48 \\
 \midrule
\multirow{8}{*}{(\texttt{o})} & \textit{00824} & 1 & 10 &  &  &  & & \\
 & \textit{00829} & 1 & 7 & &  &  &  & \\
 & \textit{00843} & 2 & 13 & &  &  & & \\
 & \textit{00861} & 2 & 24 & &  &  &  & \\
 & \textit{00862} & 3 & 36 & &  &  &  & \\
 & \textit{00873} & 2 & 11 & &  &  &  & \\
 & \textit{00877} & 2 & 13 & &  &  &  & \\
 & \textit{00890} & 2 & 11 & &  &  &  & \\
  \cmidrule{2-9}
  & \textit{Overall} &  & & & - & - & - & \\
\bottomrule
\end{tabular}
\footnotesize
Evaluation of 20 frequent distinct object categories. Success rate criterium: $\text{IoU}>0.25$. The floor and room counts refer to the ground-truth labels. mean/median/max-SR denotes when queried for a room whether the mean/median/max across all room emb vs query rooms is taken. This score is used to select the most appropriate rooms given a query. The max-value works better on larger scenes while median works better on smaller scenes. 
\red{Call it Graph Querying as above. FYI the number of trials is lower for (o,r) compared to (o,r,f) because we observe a higher number of duplicates whenever we drop the floor specification.}
\end{threeparttable}
\label{tab:real-world-retrievel}
\end{table}

\begin{table}[t]
\centering
\scriptsize
\caption{Object-Level Semantics Evaluation on HM3DSem}
\setlength\tabcolsep{3pt}
\begin{threeparttable}
\begin{tabular}{cc|cccccc|c}
 \toprule

Method & Scene  & $top_{5}$ & $top_{10}$ & $top_{25}$ & $top_{100}$ & $top_{250}$ & $top_{500}$ & AUC$_{k}^{top}$ \\
\midrule
\midrule
 \multirow{9}{*}{\rotatebox[origin=c]{90}{VLMaps \cite{huang23vlmaps}}} & \textit{00824} & 0.0 & 0.0 & 0.0 & 15.21 & 22.16 & 34.79 & 54.39 \\
  & \textit{00829}  &  0.0 & 0.0 & 0.0 & 19.18 & 34.29 & 48.98 & 61.36 \\
& \textit{00843}  &  0.0 & 0.0 & 0.0 & 15.52 & 27.16 & 45.07 & 57.43 \\
& \textit{00861}  &  0.0 & 0.0 & 1.29 & 18.74 & 29.98 & 44.03 & 60.05 \\
& \textit{00862}  &  0.0 & 0.0 & 0.0 & 17.1 & 25.3 & 37.6 & 56.12 \\
& \textit{00873} & 0.22 & 0.67 & 1.78 & 15.56 & 22.89 & 34.89 & 52.89 \\
& \textit{00877} & 0.2 & 0.4 & 0.6 & 14.0 & 26.8 & 37.4 & 54.03 \\
& \textit{00890} & 0.0 & 0.31 & 0.62 & 7.23 & 19.54 & 37.38 & 53.35 \\
\cmidrule{2-9}
& Overall & 0.05 & 0.17 & 0.54 & 15.32 & 26.01 & 40.02 & 56.20  \\
 \midrule
\multirow{9}{*}{\rotatebox[origin=c]{90}{ConceptGraphs~\cite{conceptgraphs}}} & \textit{00824}  & 21.65 & 29.38 & 35.57 & 57.47 & 72.16 & 82.22 & 84.41 \\ 
 & \textit{00829} & 16.73 & 22.86 & 35.10 & 58.37 & 75.51 & 83.67 & 86.00 \\ 
 & \textit{00843} & 15.52 & 20.30 & 27.76 & 51.34 & 68.96 & 79.10 & 82.05 \\ 
 & \textit{00861}  & 10.47 & 14.18 & 21.84 & 39.21 & 60.41 & 74.58 & 79.55 \\ 
 & \textit{00862} & 22.30 & 27.90 & 38.40 & 64.30 & 79.90 & 87.40 & 88.43 \\ 
 & \textit{00873} & 21.33 & 28.00 & 37.55 & 60.44 & 73.11 & 83.11 & 84.35 \\ 
 & \textit{00877} & 21.56 & 27.55 & 36.66 & 55.78 & 68.44 & 81.33 & 83.80 \\ 
 & \textit{00890} & 15.30 & 21.89 & 31.11 & 54.44 & 68.33 & 80.96 & 83.97 \\ 
\cmidrule{2-9}
& Overall & - & - & - & - & - & - & \underline{84.07} \\
 \midrule
\multirow{9}{*}{\rotatebox[origin=c]{90}{HOV-SG (ours)}}  & \textit{00824} & 21.38 & 30.59 & 40.13 & 64.14 & 75.66 & 82.24 & 86.52 \\ % peach field rlsim1
& \textit{00829} & 19.90 & 25.72 & 40.29 & 59.71 & 73.30 & 82.04 & 86.12 \\ % peach field rlsim1
& \textit{00843} & 11.31 & 16.61 & 28.62 & 46.64 & 61.48 & 72.79 & 79.23 \\ % fearless donkey rlsim1
& \textit{00861} & 11.93 & 19.49 & 28.74 & 47.39 & 62.35 & 76.47 & 81.94 \\ % fearless donkey rlsim1
& \textit{00862} & 19.49 & 27.01 & 37.18 & 57.94 & 71.50 & 81.36 & 86.17 \\ % galliant-hill rlsim1
& \textit{00873} & 21.90 & 30.79 & 41.90 & 64.44 & 78.73 & 89.20 & 88.35 \\ % 
& \textit{00877} & 23.02 & 31.54 & 39.11 & 59.62 & 70.34 & 81.80 & 85.33 \\ % genial dream rlsim1
& \textit{00890} & 18.53 & 24.11 & 35.28 & 51.78 & 66.24 & 80.96 & 85.36 \\ % genial dream rlsim1
\cmidrule{2-9}
& Overall & - & - & - & - & - & - & \textbf{84.88} \\

\bottomrule
\end{tabular}

\footnotesize
Analysis of our method's class-agnostic instance evaluation performance in terms of average precision (AP) as well as precision (P) and recall (R) on 3D masks showing an $\operatorname{IoU}>50\%$. In addition, we show the area under the top-k semantic classification curve (AUC$_{k}^{top}$ ).
\end{threeparttable}
\label{tab:seg-auc}
\end{table}
